# Supplementary material for: Beyond Item Order: Temporal Gap Tokenization for Generative Recommendation with Semantic IDs
Source: arXiv:2607.03918 source file (2026-07-04)
Supplement: Supplementary file 1 [file 06_Appendix.tex]

\section{Additional Output and Embedding Analysis}

We provide additional diagnostic analyses to further examine the behavior of ChronoSID. These results complement the main output-level analysis by inspecting paired prediction differences, token embedding structures, and the quality of the learned semantic ID codebook.

\begin{table}[t]
\centering
\vspace{-1em}
\caption{Paired output comparison between ReSID and ChronoSID. ``ReSID only'' denotes test instances that are correctly predicted by ReSID but missed by ChronoSID, while ``ChronoSID only'' denotes the opposite case.}
\label{tab:paired_output_analysis}
\vspace{-0.8em}
\small
\setlength{\tabcolsep}{6pt}
\begin{tabular}{lcccc}
\toprule
\textbf{Metric} & \textbf{ReSID only} & \textbf{ChronoSID only} & \textbf{Net Gain} & \textbf{McNemar $p$-value} \\
\midrule
Hit@5  & 725  & 881  & +156 & $1.09 \times 10^{-4}$ \\
Hit@10 & 1031 & 1207 & +176 & $2.15 \times 10^{-4}$ \\
\bottomrule
\end{tabular}
\vspace{-1em}
\end{table}

Table~\ref{tab:paired_output_analysis} shows the paired prediction differences between ReSID and ChronoSID. ChronoSID correctly recovers more instances that are missed by ReSID than the reverse direction. The McNemar test further indicates that the paired improvements are statistically significant, suggesting that the gain of ChronoSID is not only reflected in aggregate metrics but also corresponds to more correct generated SID candidates on individual test cases.

\begin{figure}[t]
\centering
\includegraphics[width=0.9\linewidth]{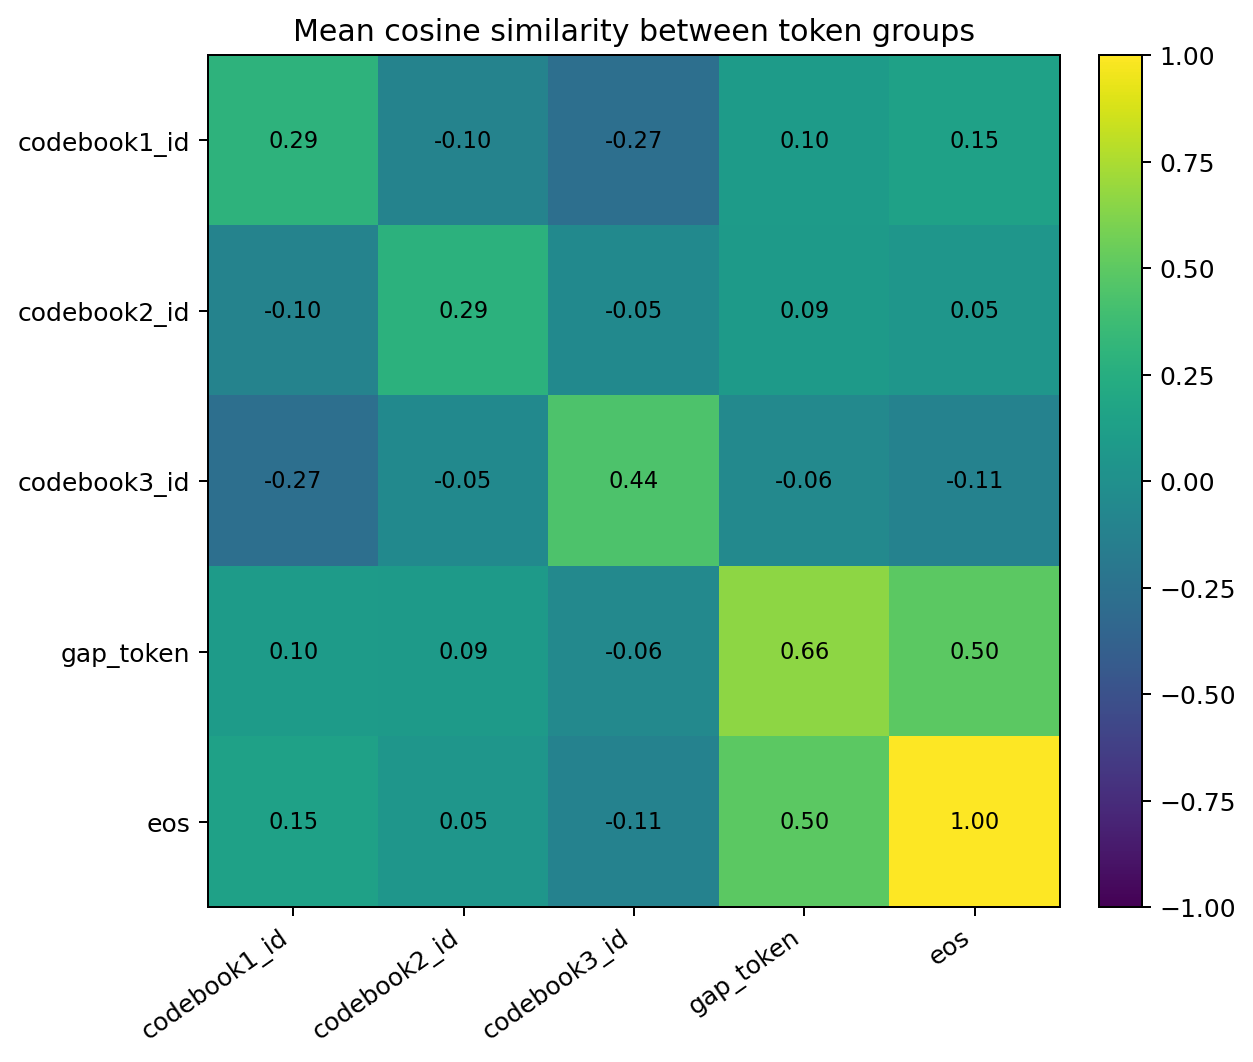}
\vspace{-0.8em}
\caption{Block-wise cosine similarity among learned T5 token embeddings. Gap tokens form a coherent token group and remain distinguishable from semantic codebook tokens, indicating that temporal tokens are learned as meaningful symbolic inputs.}
\label{fig:t5_token_block_cosine}
\vspace{-1em}
\end{figure}

Figure~\ref{fig:t5_token_block_cosine} further analyzes the learned token embedding space through block-wise cosine similarity. The gap-token group shows high internal similarity, while its similarity to semantic codebook tokens is much lower. This observation is consistent with the PCA visualization in the main text and suggests that the model learns a distinguishable representation structure for temporal gap tokens rather than treating them as arbitrary additional tokens.

\begin{figure*}[t]
\centering
\begin{minipage}{0.32\textwidth}
    \centering
    \includegraphics[width=\linewidth]{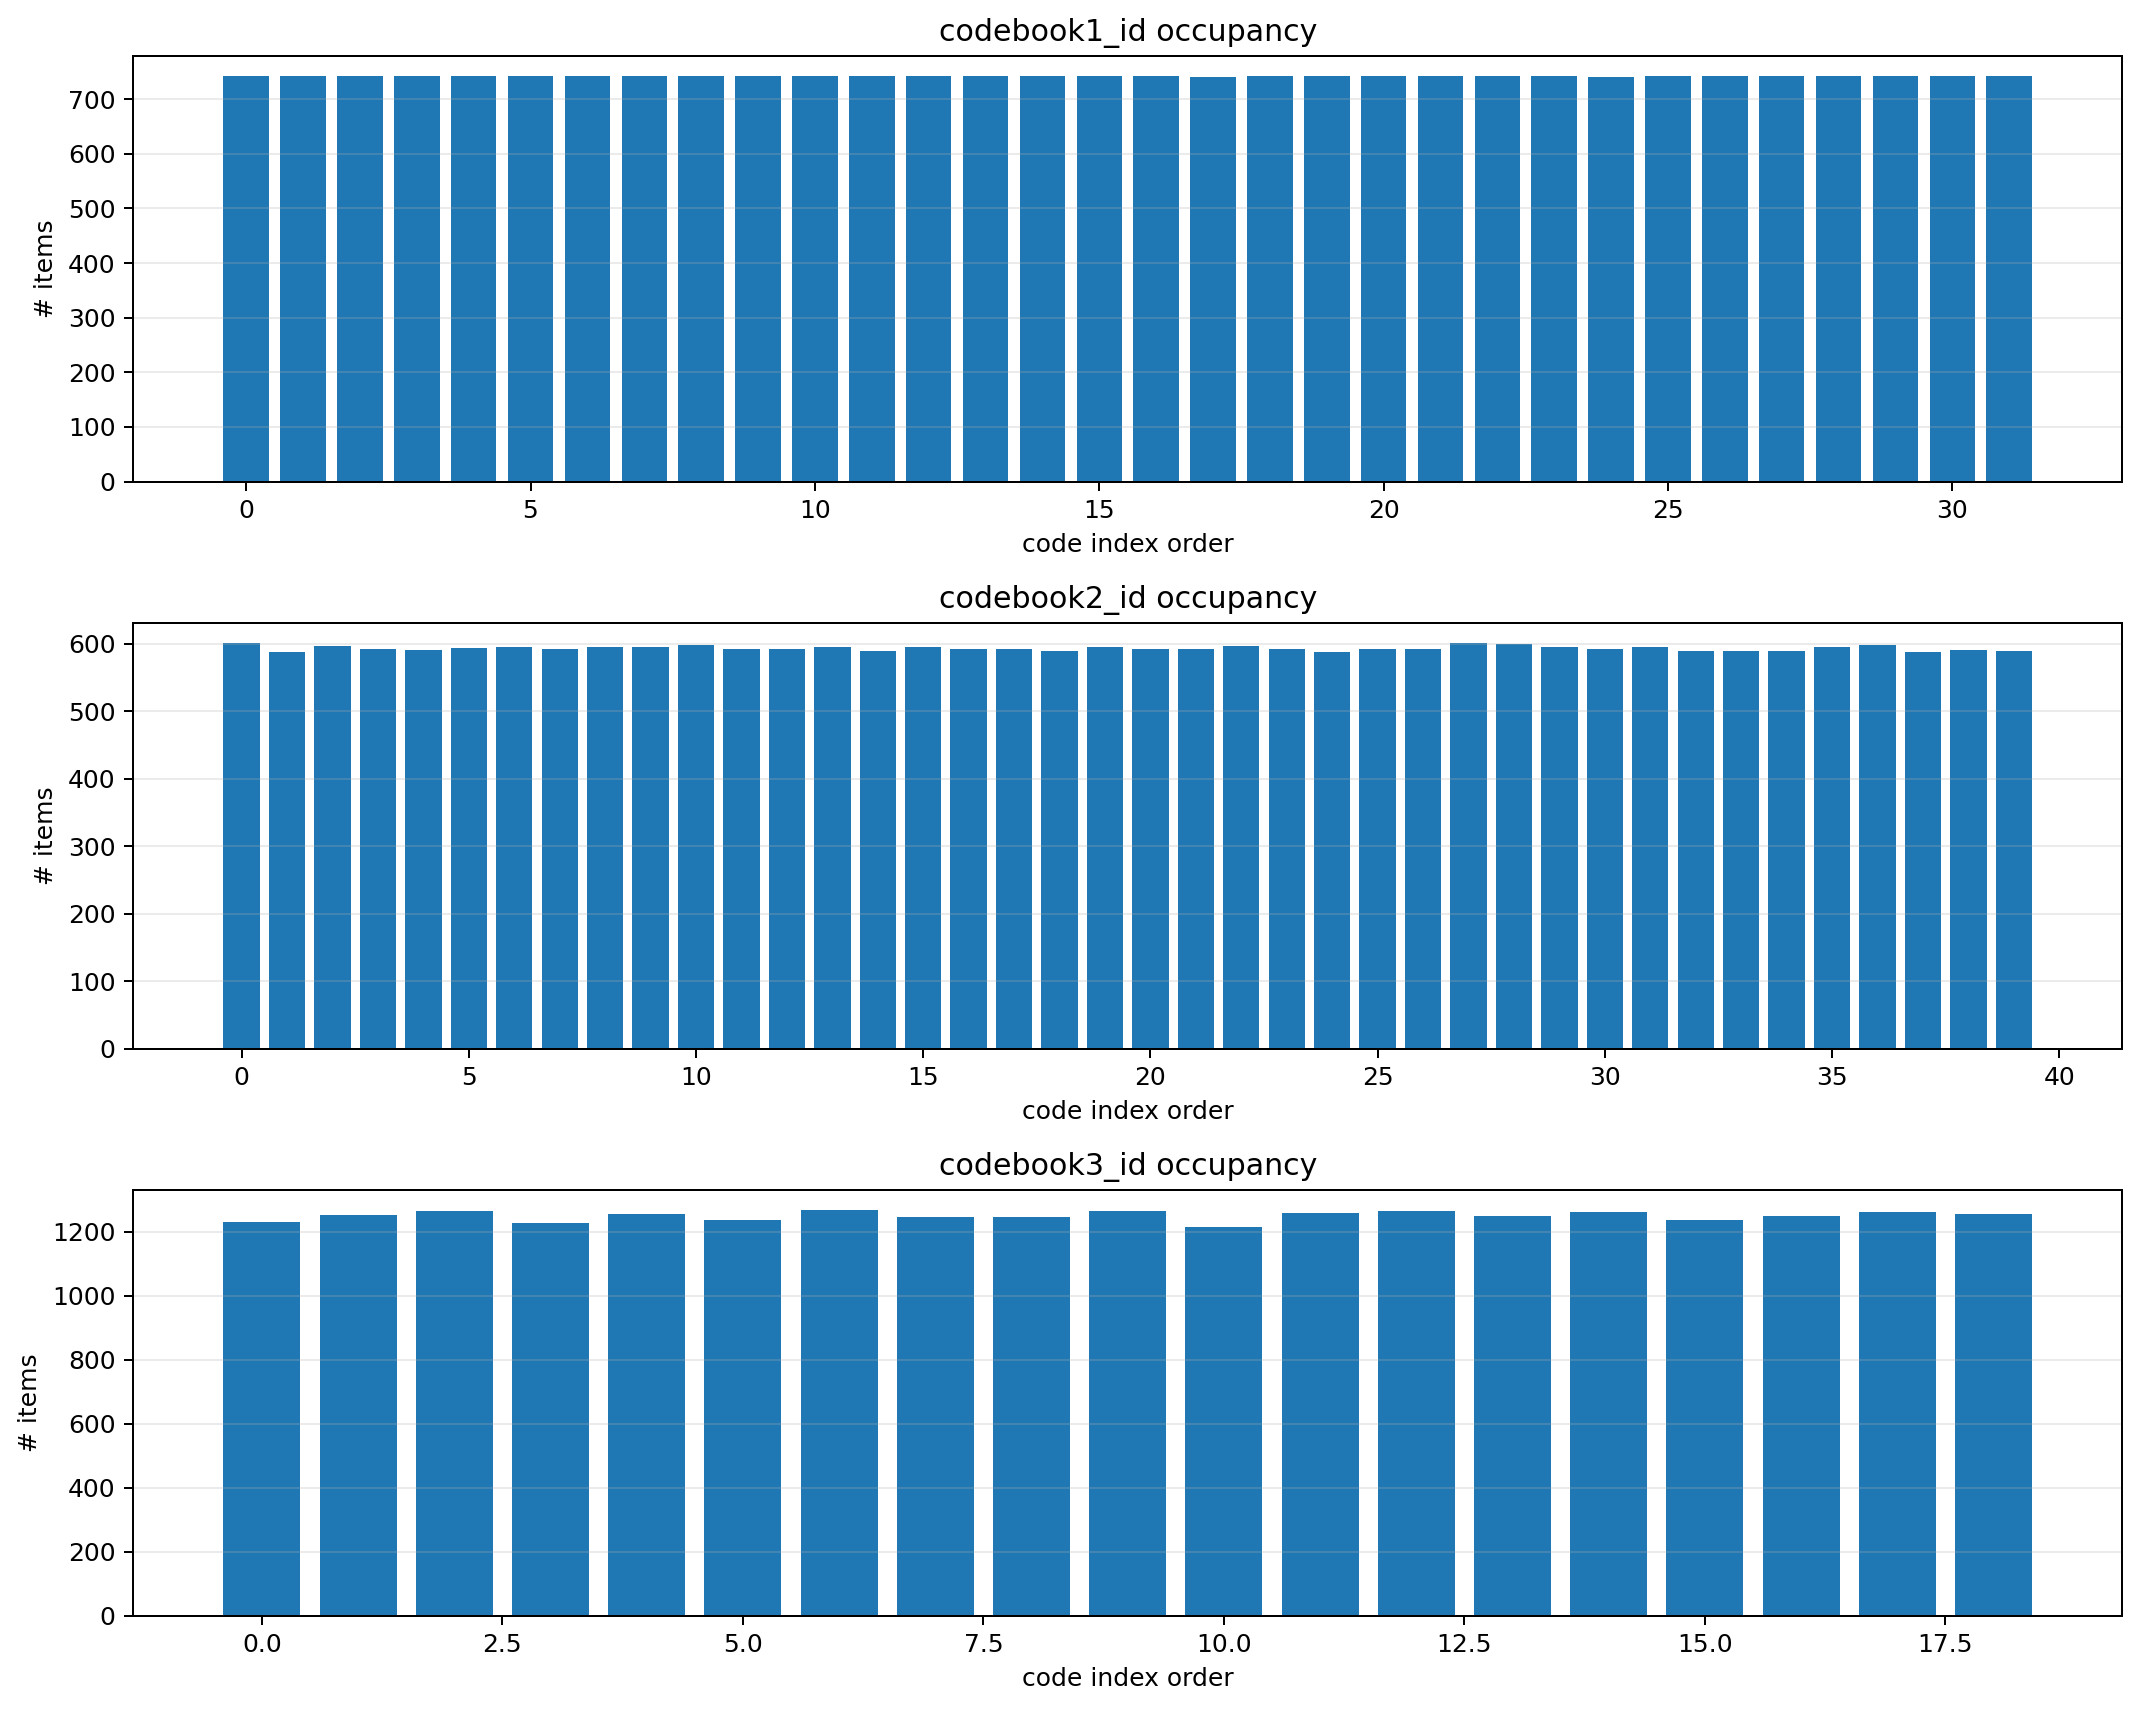}
\end{minipage}
\hfill
\begin{minipage}{0.32\textwidth}
    \centering
    \includegraphics[width=\linewidth]{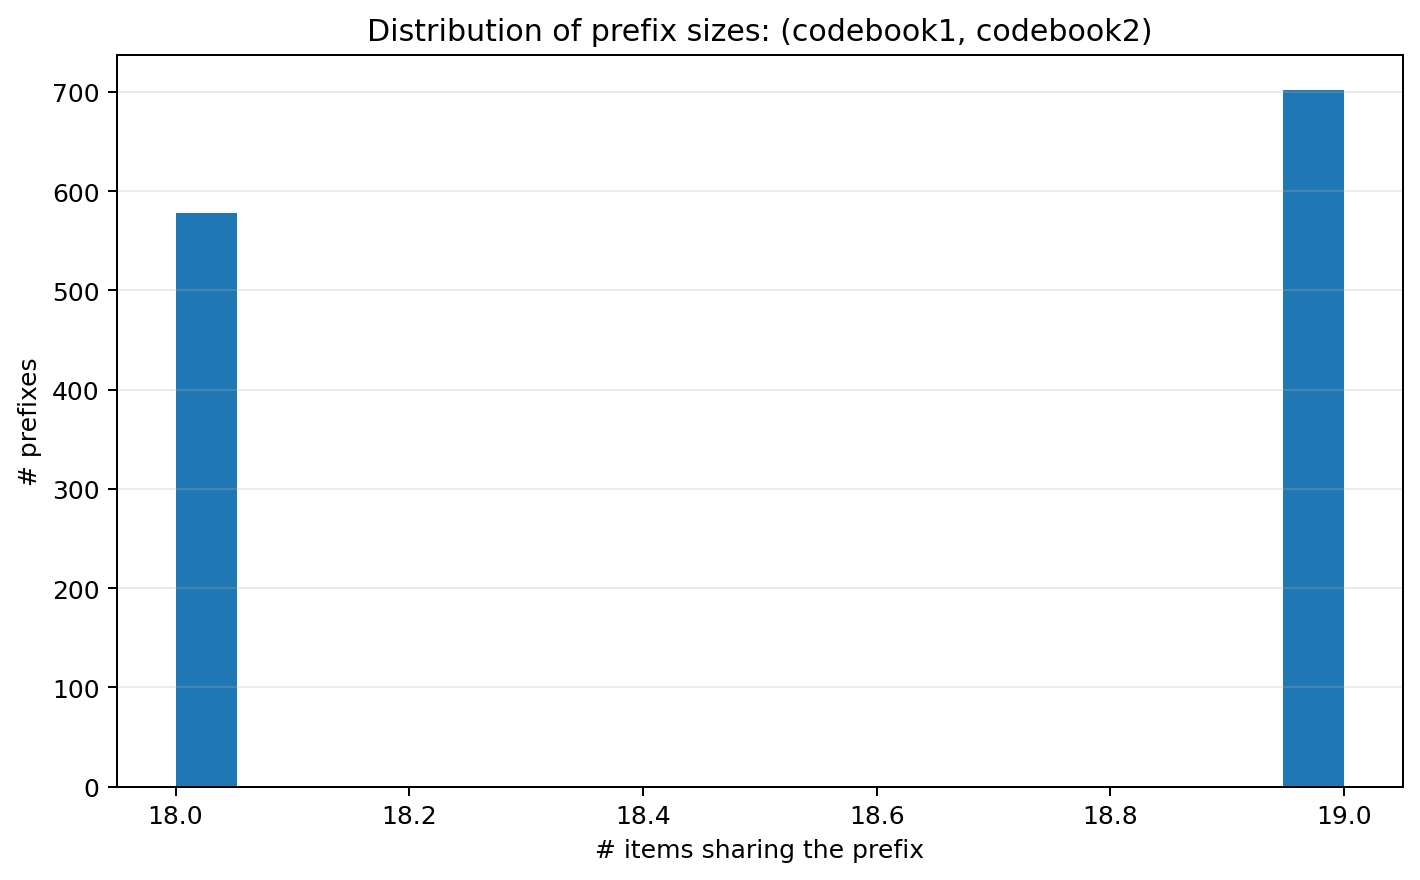}
\end{minipage}
\hfill
\begin{minipage}{0.32\textwidth}
    \centering
    \includegraphics[width=\linewidth]{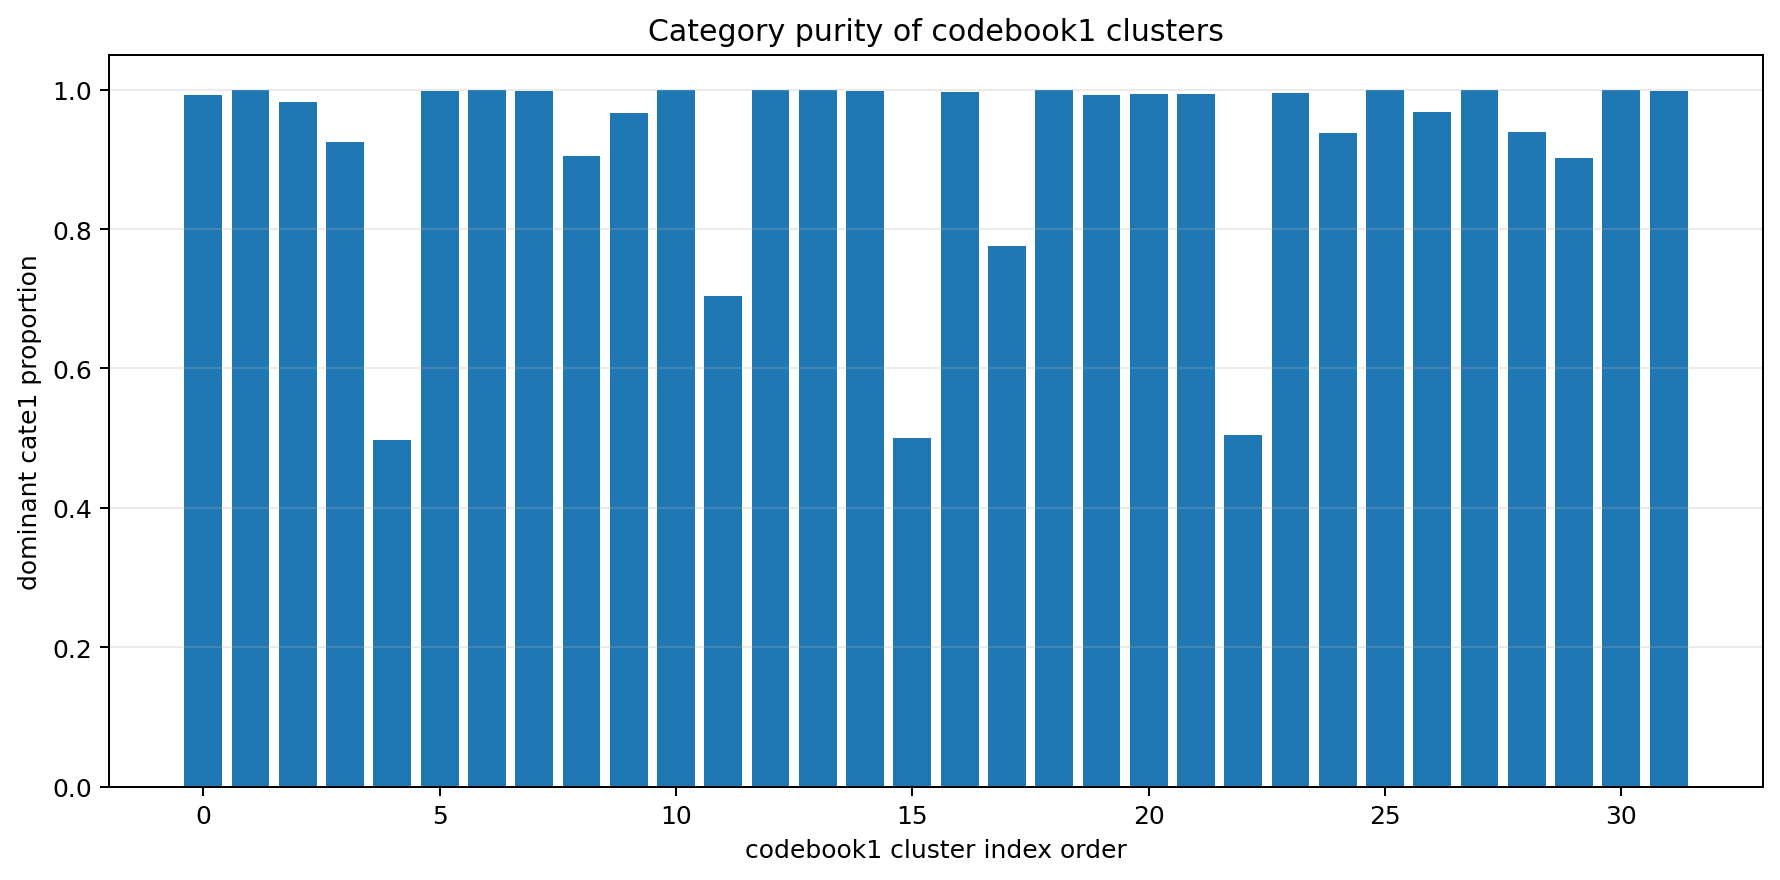}
\end{minipage}
\vspace{-0.8em}
\caption{Additional semantic ID codebook diagnostics. Left: code usage at different codebook levels. Middle: distribution of item counts under each $(c_1, c_2)$ prefix. Right: category purity of level-1 code clusters.}
\label{fig:codebook_diagnostics}
\vspace{-1em}
\end{figure*}

We also examine the learned semantic ID codebook in Figure~\ref{fig:codebook_diagnostics}. The codebook occupancy plot shows that the semantic codes are effectively used without severe collapse. The prefix-size distribution further indicates that item assignments under $(c_1, c_2)$ prefixes are well balanced, which is important for maintaining the scalability and uniqueness of semantic ID generation. In addition, the level-1 category purity analysis shows that the learned coarse codes are semantically meaningful and align well with item category structure.

Overall, these additional analyses provide supporting evidence from different perspectives. ChronoSID generates more correct SID candidates at the paired-output level, learns coherent and distinguishable temporal token embeddings, and preserves a balanced and semantically meaningful codebook structure.
